# Supplementary material for: Optimisation in Neurosymbolic Learning Systems
Source: arXiv:2401.10819 source file (2024-01-19)
Supplement: Supplementary file 1 [file appendix_experiments.tex]

In this Appendix, we report additional experiments on the \pred{same} problem. 
Throughout this Appendix we use vanilla stochastic gradient descent with a learning rate of 0.01 and 0.5 momentum instead of ADAM. 
The reason for this is that the best configurations seem to perform better with this optimizer, while the other configurations seem to perform better with ADAM. 

\subsection{Varying the Aggregators}
\label{sec:mnist_symmetric_aggregator}
In this section, we analyze symmetric configurations in the \pred{same} problem, except that we use aggregators other than the one formed by extending the t-norm. In particular, we will consider the RMSE aggregator ($A_{GME}$ with $p=2$) and the log-product aggregator $\logprod$.

\begin{table}[h]%{r}{0.53\linewidth}
\centering
\begin{tabular}{l....|....}
    &  \multicolumn{4}{c}{$\logprod, w_{\dfl}=10$} & \multicolumn{4}{c}{$A_{RMSE}, w_{\dfl}=1$} \\
\hline 
\multicolumn{1}{l}{}     & \mc{Accuracy} & \mc{$\mpratio$} & \mc{$\mpupdateratio$} & \mc{$\mtupdateratio$} & \mc{Accuracy} & \mc{$\mpratio$} & \mc{$\mpupdateratio$} & \mc{$\mtupdateratio$}               \\
\hline
 $T_G$        & 96.3          & 0.10            & \bft{0.89}            & 0.97 \
                                    & 96.2          & 0.10            & \bft{0.89}            & 0.97                           \\
 $T_{LK}$     & 96.6          & 0.5             & 0.33                  & 0.67                           
                                    & 96.9          & 0.5             & 0.06                  & 0.95                           \\
                     $T_P$        & \bft{96.7}    & 0.44            & 0.48                  & 0.69                           
                     & \bft{97.0}    & 0.08            & 0.81                  & 0.98 \\
                     $T_Y,\ p=2$  & 96.4          & 0.40            & 0.54                  & 0.74                           
                     & 96.6          & 0.12            & 0.87                  & 0.97                           \\
                     $T_Y,\ p=20$ & 96.0          & 0.29            & 0.51                  & 0.78                           
                     & 95.9          & 0.18            & 0.82                  & 0.98                           \\
                     $T_{Nm}$     & 95.4          & 0.29            & 0.44                  & 0.84                            
                     & 95.4          & 0.03            & 0.62                  & \bft{0.99}                           \\

                      % $T_H, v=0$  & 11.9          & 0.66            & 0.88                  & 0.10                           \\
                      % $T_T$       & 12.0          & ?               & ?                     & ?                             \\
\hline
\end{tabular}
\caption{Configurations using the RMSE aggregator with $w_{\dfl}=1$ and the log product aggregator with $w_{dfl}=10$.}
\label{table:mnist_symmetric_rmse}
\end{table}

Table \ref{table:mnist_symmetric_rmse} shows the results when using the RMSE aggregator and a \dfl weight of 1 and the log product aggregator and a \dfl weight of 10. 
% We note that these experiments were run with the basic SGD algorithm with a learning rate of 0.01 and a momentum value of 0.5. 
Nearly all configurations perform significantly better using these aggregators than when using their `symmetric' aggregator. In particular, the Gödel, \luk\ and Yager t-norms all outperform the baseline with both aggregators as they are differentiable everywhere and can handle outliers.

The product t-norm seems to do slightly worse with the RMSE aggregator than with the log-product aggregator. Like we discussed in Section \ref{sec:prod-implication}, $\mpratio$ is higher using this aggregator because the corners $a_i=0,\ c_i=0$ and $a_i=1,\ c_i=1$ will have no gradient when using the RMSE aggregator.
%By Equation \ref{eq:deriv_apme} we find that the derivative of $A_{RMSE}$ is $\frac{1 - x_i}{n\sqrt{\frac{1}{n}\sum_{j=1}^n(1 - x_j)^2}}$. In this context, $x_i$ is the truth value of the implication. The reason the Reichenbach implication is so imbalanced is because there is a gradient of almost 1 into the antecedent around $a_i=0$, $c_i=0$ (as $\dmta_{I_{RC}} = 1-c$). However, $1-x_i$ is going to be around 0 as $1 - a_i + a_i\cdot c_i \approx 1$. Thus, the derivative around $a_i=0$, $c_i=0$ is also around 0 as these will get multiplied. The derivative of the log-product aggregator however is $\frac{1}{x_i}$, which is around 1 if the implication is true. So, the gradient going into the antecedent $a_i$ is also around 1. This explains the stark contrast of the values of $\mpratio$ between the two aggregators.
However, the values of $\mpupdateratio$ and $\mtupdateratio$ are much lower than when using the log-product aggregator. This could have to do with the previously made point: As it no longer has a gradient of 1 at the corners $a=0,\ c=0$ and $a=1,\ c=1$, the large gradients are only when the agent is not yet confident about some prediction. This case is inherently `riskier', but also contributes more information. It is not as informative to increase the confidence of $a=0$ if $a$ is already very low.% Still, it is surprising to see that the value of $\mtupdateratio$ seems to be worse than random guessing when using $A_{RMSE}$.

% \begin{wraptable}{r}{0.53\linewidth}
% \begin{tabular}{l....}
% \hline
%             & \mc{Accuracy} & \mc{$\mpratio$} & \mc{$\mpupdateratio$} & \mc{$\mtupdateratio$}               \\
% \hline
% $T_G$       & 96.2          & 0.10            & \bft{0.89}            & 0.97                           \\
% $T_{LK}$    & 96.9          & 0.5             & 0.06                  & 0.95                           \\
% $T_P$       & \bft{97.0}    & 0.08            & 0.81                  & \bft{0.98} \\
% $T_Y, p=2$  & 96.6          & 0.12            & 0.87                  & 0.97                           \\
% $T_Y, p=20$ & 95.9          & 0.18            & 0.82                  & 0.98                           \\
% % $T_H, v=0$  & 11.9          & 0.66            & 0.88                  & 0.10                           \\
% % $T_T$       & 12.0          & ?               & ?                     & ?                             \\
% \hline
% \end{tabular}
% \caption{Symmetric configurations using the log-product aggregator. For all the results we use $w_1=10$.}
% \label{table:mnist_symmetric_cross_entropy}
% \end{wraptable}

The \luk\ t-norm has a particularly high accuracy of 96.9\% with the log product and is on the level of performance of the product t-norm. However, it has a very low value for $\mpupdateratio$ of 0.06 and a relatively low value for $\mtupdateratio$. Interestingly, it is also the only configuration for which $\mpupdateratio$ is higher when using the RMSE aggregator than the log-product aggregator. %The Gödel and Yager norms have slightly higher accuracy, although it seems to be less stable judging by the end accuracy.  Neither the Hamacher nor the trigonometric t-norms are able to surpass the baseline at all. The Hamacher t-norm is interesting in that it has both a high value of $\mpratio$ and $\mpupdateratio$, which is unique in the experiments. However, it also has an extremely low value for $\mtupdateratio$ of 0.1, which is far lower than guessing randomly. The trigonometric t-norm clearly destabilizes the results with these aggregators as well. 
