# Supplementary material for: Optimisation in Neurosymbolic Learning Systems
Source: arXiv:2401.10819 source file (2024-01-19)
Supplement: Supplementary file 2 [file ilr.tex]

% \section{Dual Problem}
% This section introduces a dual problem to Equation \ref{eq:optim-problem}. This is used extensively in several proofs. 




% \section{Schur-concave t-norms (Proofs)}
% \label{appendix:schur-concave}

% \subsection{Minimal \boost\ function for t-norms}
% \label{appendix:boost-schur-tnorm}

% \begin{theorem}
%     \label{theorem:schur-concave-t-norm}
%     Let $T$ be a Schur-concave t-norm that is strictly cone-increasing at $\revis{T}$ and let $\|\cdot \|$ be a strict norm. Then there is a minimal \boosted\ vector $\minboostv$ for $\truth$ and $\revis{T}$ such that whenever $\truths_i> \truths_j$, then $\minboosts_i - \truths_i\leq \minboosts_j - \truths_j$. 
% \end{theorem}

% \subsection{Closed-form \boost\ function using additive generators}
% \label{appendix:closed-form-additive}
% \begin{proposition}
%     \label{prop:additive-generator}
%     Let $T$ be a Schur-concave t-norm with additive generator $g$ and let $0<\revis{T}\in [T(\truth, \truthc), \revismax{T}]$. 
%     Let $K\in \{0, ..., n-1\}$ denote the number of truth values such that $\minboosts_i=\truths_i$ in Equation \ref{eq:minboost-t-norm-schur-concave}.
%     % Let $N\subseteq \{1, ..., n\}$ be the set of indices $i$ such that the $\minboostv$ from Equation \ref{eq:minboost-t-norm-schur-concave} has $\minboosts_i=\truths_i$. 
%     Then using

%     \begin{equation}
%         \lambda_K = g^ {-1}\left(\frac{1}{n-K}\left(g(\revis{T}) -\sum_{i=1}^K g(\truths^\downarrow_i) - \sum_{i=1}^m g(C_i)\right)\right)
%     \end{equation}

%     in Equation $\ref{eq:minboost-t-norm-schur-concave}$ gives $T(\minboostv, \truthc)=\revis{T}$ if $\minboostv\in [0, 1]^n$. 
% \end{proposition}




% \subsection{$L_1$ minimal \boost\ function for t-norms}
% \label{appendix:boost-schur-t-norm-L1}
% \begin{proposition}
%     Let $\truth\in [0, 1]^n$ and let $T$ be a Schur-concave t-norm that is strictly cone-increasing at $\revis{T}\in [T(\truth, \truthc), \revismax{T}]$. Then there is a value $\lambda\in [0, 1]$ such that the vector $\minboostv$,
%     \begin{equation}
%         \label{eq:minboost-t-norm-schur-concave}
%         \minboosts_i = \begin{cases}
%             \lambda, & \text{if } \truths_i < \lambda, \\
%             \truths_i, & \text{otherwise,}
%         \end{cases}
%     \end{equation}
%     is a minimal \boosted\ vector for $T$ and the $L_1$ norm at $\truth$ and $\revis{T}$.
% \end{proposition}


% \subsection{$L_1$ minimal \boost\ function for t-conorms}
% \label{appendix:schur-concave-t-conorm-l1}
% \begin{proposition}
%     Let $\truth\in [0, 1]^n$ and let $S$ be a Schur-convex t-conorm that is strictly cone-increasing at $\revis{S}\in [S(\truth, \truthc), 1]$. Then there is a value $\lambda\in [0, 1]$ such that the vector $\minboostv$,
%     \begin{equation}
%         \minboosts_i = \begin{cases}
%             \lambda & \text{if } i={\arg\max}_{i\in D}\truths_i, \\
%             \truths_i, & \text{otherwise,}
%         \end{cases}
%     \end{equation}
%     is a minimal \boosted\ vector for $S$ and the $L_1$ norm at $\truth$ and $\revis{S}$.
% \end{proposition}
% \begin{proposition}
%     Let $\truth\in [0, 1]^n$ and let $S$ be a Schur-convex t-conorm that is strictly cone-increasing at $\revis{S}\in [S(\truth, \truthc), 1]$. Then there is a value $\lambda\in [0, 1]$ such that the vector $\minboostv$ with $i\in D$,
%     \begin{equation}
%         \minboosts_i = \begin{cases}
%             \lambda & \text{if } i={\arg\max}_{i\in D}\truths_i, \\
%             \truths_i, & \text{otherwise,}
%         \end{cases}
%     \end{equation}
%     is a minimal \boosted\ vector for $S$ and the $L_1$ norm at $\truth$ and $\revis{S}$.
% \end{proposition}



% \subsection{$L_1$ minimal \boost\ function for residuums}
% \label{appendix:boost-schur-residuum}
% \todo{This doesn't consider constants}
%     \begin{proposition}
%         Let $\truths_1, \truths_2\in [0,1]$ and let $T$ be a strict Schur-concave t-norm with additive generator $g$. Consider its residuum $R(\truths_1, \truths_2)=\sup \{z\vert T(\truths_1, z)\leq \truths_2\}$ that is strictly cone-increasing at $0<\revis{R}\in [R(\truths_1, \truths_2), \revismax{R}]$. Then there is a value $\lambda\in [0, 1]$ such that $\minboostv=[\truths_1, \lambda]^\top$ is a minimal \boosted\ vector for $R$ and the $L_1$ norm at $\truth$ and $\weight$. 
%     \end{proposition}
    


% \section{Product t-norm with $L_2$ norm}
% \label{Appendix:product-l2}
% In this appendix, we consider the \boost\ functions for the product t-norm under the $L_2$-norm. We find that there is no simple closed-form parameterization in terms of $\revis{\varphi}$, but we can find approximations in linear time. These are satisfactory to reliably find the minimal \boost\ function.

% In the following, we wil ignore constants and consider formulas $\bigwedge_{i=1}^n P_i$, and consider the problem in Equation \ref{eq:optim-problem}. We consider the logarithm of the product as its optimum coincides. 

% \begin{equation}
%     \label{eq:optim-problem-prod-p1}
%     \begin{aligned}
%         \textrm{For all } \quad & \truth\in [0,1]^n, \revis{T_P} \in [T_P(\truth), 1] & \\
%         \min_{\boostv} \quad & \sum_{i=1}^n (\boosts_i - \truths_i)^2 & \\
%         \textrm{such that } \quad & \sum_{i=1}^n \log \boosts_i = \log \revis{T_P} \\
%         & \boosts_i-1 \leq 0 
%     \end{aligned}
% \end{equation}
% With Lagrangian $L=\sum_i (\boosts_i - \truths_i)^2 + \lambda(\sum_i \log \boosts_i -\log \revis{T_P})  - \gamma_i(\boosts_i - 1)$, and so
% \begin{align*}
%     \frac{\partial L}{\partial \boosts_i} &= 2(\boosts_i - \truths_i) - \gamma_i +\frac{\lambda}{\boosts_i}=0 \\
%     \lambda &= (\gamma + 2\truths_i - 2\boosts_i) \boosts_i %(\gamma_i-2\boosts_i)(\truths_i + \boosts_i)
% \end{align*}
% Since this holds for all $i$, we find that for all $i$, $j$, $(\gamma + 2\truths_i - 2\boosts_i) \boosts_i= (\gamma + 2\truths_j - 2\boosts_j) \boosts_j=\lambda$. We partition $\{1, ..., n\}$ into sets $I$ and $M$, where $I$ contains all $i$ such that $\boosts_i < 1$, and $M$ those where $\boosts_i=1$. For $i\in I$, by noting that using the complementary slackness condition $\gamma_i=0$, this induces a quadratic equation in $\boosts_i$ with solutions
% \begin{equation}
%     \label{eq:boostv_p2}
%     \boosts_i = \frac{1}{2}(\truths_i \pm \sqrt{\truths_i^2-2\lambda}).
% \end{equation} 
% Since we assume $\boosts_i\geq \truths_i$, we have to take the solution that adds the root of the determinant, that is, $\boosts_i=\frac{1}{2}(\sqrt{\truths_i^2-2\lambda}+\truths_i)$. Furthermore, since we constrain for $i\in I$ that $\boosts_i < 1$, we find that 
% \begin{align*}
%     1 &> \frac{1}{2}(\truths_i + \sqrt{\truths_i^2-2\lambda}) \\
%     2 - \truths_i & > \sqrt{\truths_i^2 - 2\lambda} \\
%     \lambda &> 2\truths_i - 2.
% \end{align*}
% Therefore, given some chosen value of $c$, we require for all $i\in I$ that $\lambda > 2\truths_i - 2$, and so, 
% \begin{equation*}
%     \min_{i\in I} 2\truths_i - 2 >\lambda 
% \end{equation*} 

% Unfortunately, finding the exact value of $\lambda$ such that $T_P(\boostv)=\revis{T_P}$ is a challenge. Filling in $\boosts_i$, we find
% \begin{equation}
%     T_P(\boostv)=\prod_{i=1}^n (\boosts_i)=\prod_{i\in I}\frac{1}{2}(\truths_i+\sqrt{\truths_i^2-2\lambda})=\revis{T_P}.
% \end{equation}
% This is a $2n$-th degree polynomial in $\lambda$, and we were not able to find an obvious, general closed form solution to it. Mathematica \cite{inc.MathematicaVersion12} finds a complicated closed form formula for $n=2$, but cannot find closed form formulas for $n>2$. 

% We also still need to figure out how to partition $i=\{1, ..., n\}$ into $I$ and $M$. Since $\boosts_i$ as computed by Equation \ref{eq:boostv_p2} is a strictly decreasing function in $\lambda$ for all $i\in I$, we have the following unproven proposition. It supports the result given in Theorem \ref{theorem:schur-concave-t-norm} .
% \begin{proposition}
%     For all $\lambda\in[\min_{i=1}^n 2\truths_i-2, 0]$, the function 
%     \begin{equation}
%         \minboost_{T_P}(\truth, \lambda)_i= \begin{cases}
%             \frac{1}{2}(\truths_i + \sqrt{\truths_i^2 - 2\lambda}) & \text{if } 2\truths_i -2 > \lambda, \\
%             1-\truths_i & \text {otherwise.}
%         \end{cases}
%     \end{equation}
%     has the following properties:
%     \begin{enumerate}
%         \item $\minboost_{T_P}(\truth, \lambda)$ is a minimal \boost\ vector for the product t-norm, the $L_2$ norm and $\revis{T_P}=T_P(\minboost_{T_P}(\truth, \lambda))$;
%         \item $\revis{T_P}=T_P(\minboost_{T_P}(\truth, \lambda))$ is a strictly decreasing function in $c$ on $(\min_{i=1}^n 2\truths_i-2, 0]$, and so there is a bijection between $\lambda$ and $\weight \in [T_P(\truth), 1]$ on this interval.
%     \end{enumerate}
% \end{proposition}
% % Do we have a proof for 1 yet?

% The second property is easy to see by noting the derivative of $\minboost_{T_P}(\truth, \lambda)$ is negative on $\lambda \in (\min_{i=1}^n 2\truths_i - 2]$, but for the first we do not have a direct proof as of yet and leave this for future work.

% Although $\minboost_{T_P}(\truth, \lambda)$ is not parameterized in terms of $\revis{T_P}$, it can still be used in practical scenarios where $\lambda$ can  be seen as the negative \say{confidence} in the clause. A practical implementation could learn a weight for the clause between 0 and 1, and then transform it to the domain of $\lambda$ by dividing by $\min_{i=1}^n 2\truths_i - 2$. Alternatively, $\|T_P(\truth+\minboost_{T_P}(\truth, \lambda))-\revis{T_P}\|_2$ can be minimized with respect to $\lambda$ using mathematical optimization methods like gradient descent or Newton's method to find answers in terms of $\revis{T_P}$. 


% \section{Additional experiments}
% \label{appendix:additional-experiments}
% This Appendix presents additional experiments when $\revis{\varphi}$ is not 1. 
% \subsection{Results - \Boosted\ value 0.3}
% Figures \ref{fig:results_91_0.3} and \ref{fig:results_2_0.3} present the results when the \boosted\ value $\revis{\varphi}=0.3$.
% \begin{figure}[H]
%     \includegraphics[width=\linewidth]{results_91_0.3_final.png}
%     \caption{\ale{Comparison of ILR with ADAM on uf20-91 of SATLIB. \Boosted\ value 0.3. The x-axis corresponds to the number of iterations, while the y-axis is the value of $\revis{\varphi}$ in the first row of the grid and the $L_1$ norm in the second row.}}
%     \label{fig:results_91_0.3}
% \end{figure}

% \begin{figure}[H]
%     \includegraphics[width=\linewidth]{results_20_0.3_final.png}
%     \caption{\ale{Comparison of ILR with ADAM on the uf20-91 with 20 clauses. \Boosted\ value 0.3.}}
%     \label{fig:results_2_0.3}
% \end{figure}


% \subsection{Results - \Boosted\ value 0.5}
% Figures \ref{fig:results_91_0.5} and \ref{fig:results_20_0.5} present the results when the \boosted\ value $\revis{\varphi}=0.5$. We note that the satisfaction for ADAM in \luk\ converges above 0.5 in Figure \ref{fig:results_91_0.5}. This means the final truth value is too high, and it has not found a proper solution here. 

% \begin{figure}[H]
%     \includegraphics[width=\linewidth]{results_91_0.5_final.png}
%     \caption{\ale{Comparison of ILR with ADAM on the uf20-91 of SATLIB. \Boosted\ value 0.5.}}
%     \label{fig:results_91_0.5}
% \end{figure}

% \begin{figure}[H]
%     \includegraphics[width=\linewidth]{results_20_0.5_final.png}
%     \caption{\ale{Comparison of ILR with ADAM on the uf20-91 with 20 clauses. \Boosted\ value 0.5.}}
%     \label{fig:results_20_0.5}
% \end{figure}
